# Supplementary material for: Cob: a Leaderless Protocol for Parallel Byzantine Agreement in Incomplete Networks
Source: arXiv:2108.11157 source file (2022-02-10)
Supplement: Supplementary file 1 [file Appendix.tex]

\section{Proof m-Dimensional BBA}
\labelx{appendix MBBA}
We first prove some Lemmas which will lead us to a proof of theorem \ref{mBBA_thm}.

\begin{lem}
\labelx{lem2}
If, at some step, a honest player $i$ sets $f_{i,c}=1$, then $c$-agreement will hold at the end of the step.
\end{lem}
\begin{proof}
First of all note that an honest player $i$ can set $f_{i,c}=1$ only during a Coin-Fixed-To-0 Step or a Coin-Fixed-To-1 Step, so STEP 3 is not taken under consideration.

Assume that a honest player $i$ fixes $b_{i,c}=0$ and $f_{i,c}=1$ in Coin-Fixed-To-0 Step, then, in that step, $\#_i^1(0,c) \ge 2t + 1$. This means that at least $t + 1$ honest players have sent 0 at the start of the step.
Thus, $\#_j^1(0,c) \ge t + 1$ for each other honest player $j$.
For each of these players two mutually exclusive cases may occur :
\begin{enumerate}
    \item $\#_j^1(0,c) \ge 2t + 1$. In this case $j$ sets $b_{j,c} = 0$ (and also $f_{j,c}=1$) in sub-step 1 of STEP 1.
    \item $t + 1 \le \#_j(0,c) < 2t + 1$. In this case $j$ must enter the third sub-step of STEP 1 hence sets $b_{j,c} = 0$.
\end{enumerate}
Thus $c$-agreement holds on 0 at the end the Coin-Fixed-To-0 Step.

A symmetric argument shows that $c$-agreement holds on 1 at the end of a Coin-Fixed-To-1 Step in which a honest player $i$ sets $b_{i,c}=1$ and $f_{i,c}=1$.
\end{proof}

\begin{lem}
\labelx{lem1}
For each component $c\in\{1,2,\dots,m\}$,
if at some step $c$-agreement holds, then it continues to hold in the next steps.
\end{lem}
\begin{proof}
Assume that for some component $c$ the players reached $c$-agreement at the end of some step $s$.
We want to show that in each subsequent step $c$-agreement still holds.
%Then in that step each honest player $i$ sends $\mathbf{b_i}$, so that, $\#_i^s(b_{i,c},c) \ge 2t + 1$ and thus $i$ does not change the value of component $c$ at the end of the step.
We assume that $c$-agreement has been reached on 0. A similar analysis can be done in case $c$-agreement is reached on 1. 

Let's consider the three possible options for step $s$:
\begin{itemize}
    \item if $s$ is a STEP 3 then the next step is STEP 1.
    At the beginning of STEP 1 each honest player $i$ sends its list $\mathbf{b_i}$.
    Since agreement has been reached on component $c$ during the previous step, for all honest $i$, $b_{i,c}=0$ and $\#_i^1(0,c) \ge 2t + 1$.
    This means that in STEP~1, for the component $c$, each honest player $i$ enters the first sub-step and then $c$-agreement still holds, since the component $c$ is left unchanged.

    \item if $s$ is a STEP 1 then the next step is STEP 2.
    At the beginning of STEP 2 each honest player $i$ sends its list $\mathbf{b_i}$.
    Since agreement has been reached on component $c$ during the previous step, for all honest $i$, $b_{i,c}=0$ and $\#_i^2(0,c) \ge 2t + 1$.
    This means that in STEP 2, for the component $c$, each honest player $i$ enters the second sub-step and then $c$-agreement still holds since the component $c$ is left unchanged.

    \item if $s$ is a STEP 2 then the next step is STEP 3.
    At the beginning of STEP 3 each honest player $i$ sends its list $\mathbf{b_i}$.
    Since agreement has been reached on component $c$ during the previous step, for all honest $i$, $b_{i,c}=0$ and $\#_i^3(0,c) \ge 2t + 1$.
    This means that in STEP 3, for the component $c$, each honest player $i$ enters the first sub-step and then $c$-agreement still holds since the component $c$ is left unchanged.
\end{itemize}

Thus, if $c$-agreement holds at some step, it will keep holding during the next step, and so on.
\end{proof}

%Another useful result is the following.
\begin{lem}
\labelx{lem3}
If, at the start of an execution of STEP 3, no player has yet halted and agreement has not
yet been reached on a bit list, then, being $l$ the number of list components $c$ on which $c$-agreement has not been reached, the players will be in agreement at the end of the step with probability at least $\frac{2}{3}(\frac{1}{2})^l$. 
\end{lem}

\begin{proof}
Let $\gamma$ be the current value of the counter, $P_i$ the set of players from which $i$ has received a valid message at the beginning of step 3. By the uniqueness property of
the underlying digital signature scheme, $i$ can compute $k=H({min}_{j \in P_i}H(\mult{SIG}_j(r,\gamma)))$, and then $k_1,\dots,k_m$ are well
defined.

Note that the selection of the player $p$ whose hashed digital signature is minimal is a random selection, under the assumption that $H$ is a random oracle.
This means that $p$ will be a honest player with probability at least $\frac{2}{3}$, and in this case it will propagate its message.
In particular all the honest players will receive $H(\mult{SIG}_{p}(r,\gamma))$, from which the values $k_1,\dots,k_m$ will be computed by the honest players who perform the sub-step 3 of STEP 3 of the protocol.

Let $\{c_i\}_{i=1,\dots,l}$ be the set of components of the bit list on which $c_i$-agreement does not hold and let us assume that the player $p$ is honest.\\

For each component $c_i$ of the bit list, notice that it is impossible that some honest player perform sub-step 1 and some sub-step 2 of STEP 3. In fact, being $t<\frac{1}{3}n$ the number of malicious nodes, if a node $i$ has received more than $\frac{2}{3}n$ messages for 1 and a node $j$ has received more than $\frac{2}{3}n$ messages for 0, then $i$ has received at least $\frac{2}{3}n-t>\frac{1}{3}n$ messages for 1 from honest nodes, and such messages have reached also $j$. However, $j$ has received at least $\frac{2}{3}n$ messages for 0, which is a contradiction since $\frac{2}{3}n+\frac{2}{3}n-t>n$, and $j$ can not receive more than $n$ messages from distinct nodes.\\

Therefore there are five exhaustive cases that must be considered and may lead the honest players to $c_i$-agreement:
\begin{itemize}
    \item All honest players update their binary $c$ component according to sub-step 1 of STEP 3.\\
    In this case $c$-agreement hols on 0.
    
    \item All honest players update their binary $c$ component according to sub-step 2 of STEP 3.\\
    In this case, $c$-agreement holds on 1.
    
    \item All honest players update their binary $c$ component according to sub-step 3 of STEP 3.\\
    In this case, at the end of Step 3, $c$-agreement holds on $k_c$.
    
    \item Some honest players update their binary $c$ component according to sub-step 1 of STEP 3 and all others according to sub-step 3 of STEP 3.\\
    The honest players updating the value according to sub-step 1 will set the component $c$ of their list to 0, while the ones updating their $c$ component according to sub-step 3 will set it to $k_c$ which is 0 with probability $\frac{1}{2}$.
    This means that $c$-agreement is reached on 0 with probability $\frac{1}{2}$.
    
    \item Some honest players update their binary $c$ component according to sub-step 2 of step 3 and all others according to sub-step 3 of STEP 3.\\
    The honest players updating the value according to sub-step 1 will set the component $c$ of their list to 1, while the ones updating their $c$ component according to sub-step 3 will set it to $k_c$ which is 1 with probability $\frac{1}{2}$.
    This means that $c$-agreement is reached on 1 with probability $\frac{1}{2}$.
\end{itemize}

When the player $p$ is honest, we can assume that the values $k_c$ are chosen randomly and independently, under the assumption that $H$ is a random oracle (\cref{RO}). Hence at the end of STEP 3 the players will reach $c$-agreement for all values of $c \in \{1,\dots,m\}$, which means agreement, with probability at least $(\frac{1}{2})^l$.
Thus, given that the probability of having the player $p$ honest is $(\frac{2}{3})$ we can conclude that anytime the players reach STEP 3 of the protocol, before the end of the step they will be in agreement with probability at least $(\frac{2}{3})(\frac{1}{2})^l$. 
%In fact if $p$ is malicious, it can decide to send a message only to some player, so the honest players entering sub-step 3 of STEP 3 may select different minimal hashed signatures of message $(r,\gamma)$, updating with different bits their $c$-th component.
\end{proof}

We now can prove \cref{mBBA_thm}.
\begin{proof}
We must prove the following properties that characterize a Byzantine agreement protocol with soundness $\sigma=1$.
\begin{enumerate}
    \item \labelx{Halt} All honest players HALT with probability 1.
    
    This is true since agreement is reached with probability 1.
    In fact, if at the beginning of STEP 3 the players are not in $c$-agreement over $l$ components, with probability  $\ge \frac{2}{3} (\frac{1}{2})^l > 0$ they will be in agreement at the end of that step, hence with the growing of the number of STEP 3 executions the probability to reach agreement converges to 1. Note that at every STEP 3 execution, the number of components not agreed upon can not increase, so the probability to end the protocol in the next STEP 3 execution can not decrease.
    
    Once agreement is reached, the honest players will HALT in the following 2 steps since it will finalize the zeroes in STEP~1 and the ones in STEP 2 (updating the locally saved list $\mathbf{f}$ with ones corresponding to the finalized components).
    
    \item $out_i = out_j$ for all honest players $i$ and $j$.
    
    This is true because by point \ref{Halt} all honest players halt, thus they have $\mathbf{f}=\mathbf{1}$ and by applying \Cref{lem2} to every component we can conclude that they are in agreement.
    
    \item If the initial value of every honest players $i$ is a list $\mathbf{b_i}=\mathbf{b}$, then $out_i=\mathbf{b}$ for every honest player $i$.
    
    It is exhaustive to consider the following two cases.
    \begin{itemize}
        \item if $\mathbf{b}$ is the list of all zeros, then all honest players enter sub-step 1 of STEP 1 and when they verify the EXIT CHECK, once they have updated all their components, they will halt setting $out_i=\mathbf{b}$.
        
        \item Otherwise during STEP 1, for all $c \in \{1,2,\dots,m\}$ if $b_{i,c}=0$ they will set $b_{i,c}=0$ updating $\mathbf{f}$ setting $f_{i,c}=1$, but will not halt since for some $c$ we have $b_{i,c}=1$.
        These components $c$ will be finalized during STEP 2 when it will be set $b_{i,c}=1$ and $f_{i,c}=1$.
        In this case, once the last coordinate is updated the EXIT CHECK will be verified, every honest player $i$ will output $out_i=\mathbf{b}$.
    \end{itemize}
\end{enumerate}
\end{proof}

\section{Proof m-Dimensional GC}
\labelx{Appendix MGC}
We provide a proof for \cref{mGC_thm}
\begin{proof}
    The analysis is performed on a generic component $c$, and the final result is a consequence of the properties holding on every component. \\
    \begin{enumerate}
        \item We first prove that it is impossible for two honest players $i$ and $j$ to end the protocol with the $c$-th output component $(v_{i,c},g_{i,c})$ and $(v_{j,c},g_{j,c})$, with $\lvert g_{i,c}-g_{j,c} \rvert = 2$.
	
        Let us assume $g_{i,c}=0$ (hence $v_{i,c}=\bot$) and $g_{j,c}=2$ (hence $v_{j,c}\ne\bot$).
        This means that, at the end of STEP 2, $\#_j^2(v_j,c)\ge \lfloor\frac{2n}{3}\rfloor+1$, out of these messages, the honest players have sent at least
        $        \lfloor\frac{2n}{3}\rfloor+1 - \lfloor\frac{n-1}{3}\rfloor > \frac{2n}{3} - \frac{n}{3} = \frac{n}{3}$.
        Note that $\lfloor\frac{n}{3}\rfloor+1$ is the smallest integer strictly greater than $\frac{n}{3}$, so the honest players have sent at least $\lfloor\frac{n}{3}\rfloor+1$ messages.
        Since the messages sent by honest players are received both by $j$ and by $i$, $\#_i^2(v_j,c)\ge \lfloor \frac{n}{3} \rfloor +1$ hence $g_{i,c}$ cannot be 0.
    
        \item We now prove that if $i, j$ are honest players and $g_{i,c},g_{j,c}>0$, then $v_{i,c}=v_{j,c}$.
	
	    Assume $g_{i,c},g_{j,c}>0$ and $v_{i,c}\ne v_{j,c}$.
	    This means that $\#_i^2(v_i,c)\ge \lfloor\frac{n}{3}\rfloor+1$ and $\#_j^2(v_j,c)\ge \lfloor\frac{n}{3}\rfloor+1$.
	    This means that at the beginning of STEP 2 at least two distinct honest players $h,k$ have received $\#_h^1(v_i,c)\ge \lfloor\frac{2n}{3}\rfloor+1$ and $\#_k^1(v_j,c)\ge \lfloor\frac{2n}{3}\rfloor+1$.
	
	    This is impossible since the honest players sent the same messages both to $h$ and $k$, and the number of malicious players is $\mathbf{t}\le t<\frac{n}{3}$.
	    The malicious players may have sent different messages to $h$ and $k$, but they can have sent no more than $t = \lfloor \frac{n-1}{3} \rfloor$ messages to each of the honest players.
	    Considering all the distinct messages received by either $h$ or $k$ at the end of STEP 2, we have that at most $n-\mathbf{t}$ of them have been sent by honest players, and at most $2\mathbf{t}$ by malicious players, so there are at most $n+\mathbf{t}\le n+t$ distinct messages.
	    However, we have that $2(\lfloor\frac{2n}{3}\rfloor + 1) > 2 (\frac{2n}{3}) = n + \frac{n}{3} >  n + \lfloor\frac{n-1}{3}\rfloor \ge n + t$ which contradicts the fact that the number of messages received by $h$ and $k$ can not exceed $n+t$.
	    
	    \item 
	    \begin{itemize}
	        \item We now prove that if $v'_{i,c}=v_c\ne\bot$ $\forall i \in\{1,\ldots,n\}$ for some value $v_c$, then for all honest players the output is $(v_{i,c},g_{i,c})=(v_c,2)$.
	
	    This is true because at the end of STEP 1 each honest player broadcasts $v_c$.
	    Note that the honest players are at least $n - \lfloor\frac{n-1}{3}\rfloor > n - \frac{n}{3} = \frac{2n}{3}$, and since there are an integral number of them they are at least $\lfloor\frac{2n}{3}\rfloor+1$.
	    This means that for each honest player $i$, $\#_i^1(v_c,c)\ge\lfloor\frac{2n}{3}\rfloor+1$ thus each honest player in STEP 2 broadcasts $v_c$.
	    Again for each honest player $i$ must be $\#_i^2(v_c,c)\ge\lfloor\frac{2n}{3}\rfloor+1$, and this implies $(v_{i,c},g_{i,c})=(v_c,2)$.
	    \item Finally, we prove that if  $v'_{i,c}=\bot$ $\forall i \in\{1,\ldots,n\}$ then all honest players output $(v_{i,c},g_{i,c})=(\bot,0)$.
	    In this case at the end of STEP 1 each honest player broadcasts $\bot$.
	    This means that for each honest player $i$, $\#_i^1(\bot,c)\ge\lfloor\frac{2n}{3}\rfloor+1$ thus there cannot exist a value $v_c\ne \bot$ such that $\#_i^1(v_c,c)\ge \lfloor\frac{2n}{3}\rfloor+1$ (otherwise the number of messages considered by the honest player $i$ would exceed $n$).
	    Hence $i$ will send the message with $\bot$ in $c$-th component at the end of STEP 2.
	    Again, for each honest player $i$, $\#_i^2(\bot,c)\ge\lfloor\frac{2n}{3}\rfloor+1$ thus there cannot exist a value $v_c\ne \bot$ such that $\#_i^2(v_c,c)\ge \lfloor\frac{n}{3}\rfloor+1$ and this implies $(v_{i,c},g_{i,c})=(\bot,0)$.
	    \end{itemize}
    \end{enumerate}

\end{proof}
